# Supplementary material for: Explicit Word Density Estimation for Language Modelling
Source: arXiv:2406.10256 source file (2024-06-10)
Supplement: Supplementary file 1 [file appendix.tex]

\chapter{Dummy Appendix}

You can defer lengthy calculations that would otherwise only interrupt
the flow of your thesis to an appendix.
